# Supplementary material for: Phase Transitions in Neural Networks Pruning
Source: arXiv:2602.15224 ancillary file (2026-02-16)
Supplement: Supplementary file 1 [file Supplemental_Materials.pdf]

# Supplementary Information to Phase Transitions under Neural Networks Pruning

## I. PRUNING AND RETRAINING PROCEDURE

The overall pruning and retraining procedure is summarized in Algorithm 1.

**Require:**
$\mathcal{M}$ : Starting trained model
$f_r$ : Weights fraction to remove at each step
$T, E$ : Training and Evaluation sets
**Ensure:** $m$ : Observable tracking

$m \leftarrow$ `Empty_list`
$n_w \leftarrow$ `Total_weights`$(\mathcal{M})$ ▷ Remaining weights
$n_{\texttt{rmv}} \leftarrow n_w \times f_r$ ▷ Amount of weights to remove
**while** $n_w > 0$ **do**
  $mask \leftarrow$ `Remove_weights`$(\mathcal{M}, n_{\texttt{rmv}})$
  $\mathcal{M} \leftarrow$ `Masked_train`$(\mathcal{M}, T, mask)$
  $m \leftarrow$ `Concat`$(m,$ `Evaluate`$(\mathcal{M}, E))$
  $n_w \leftarrow n_w - n_{\texttt{rmv}}$
**end while**
**return** $m$

Algorithm 1: Implemented pruning algorithm. In this pseudo-code many details have been discarded to make the process clearer.

Figure 1 shows the evolution of accuracy, prediction entropy, and outcome entropy as functions of the pruning level, defined as the fraction of remaining connections.

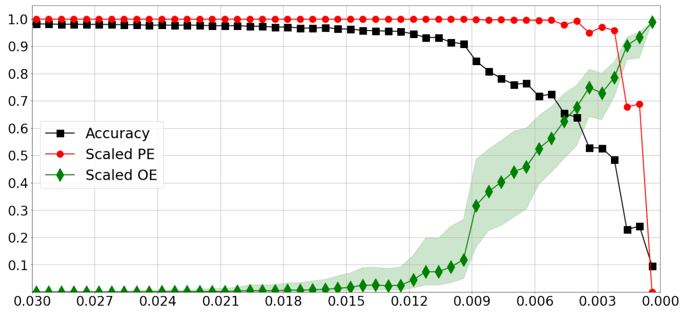


(a) CNN5 architecture on MNIST dataset.

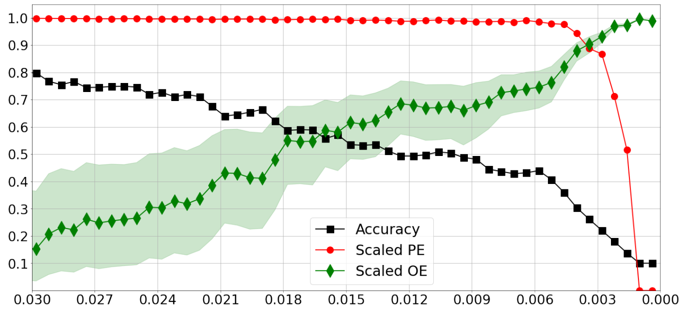


(b) CNN5 architecture on KMNIST dataset.

FIG. 1: (color on line) Analogousto the corresponding image in the main text, but for the CCN5 architecture. Detail of the behavior near the point at which the algorithm ceases to operate. The x axis shows the percentage of links remaining after pruning. From top to bottom: accuracy (black line), prediction entropy (red line) and outcome entropy (green line). Results are shown for (a) MNIST and (b) KMNIST.

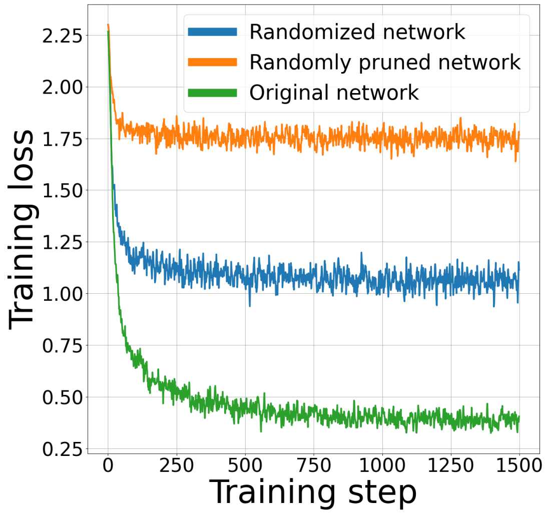


FIG. 2: (color on line) Here we show the loss in the training on y-axis with respect to the steps of training on x axis. From top to down we have (a; orange online) totally random subset of edges, (b; blue online) subset of edges self-organised in the pruning procedure and then randomized, (c; green online) the original model

In Table I and we report the estimate of these critical exponents taking into consideration that in the case the FC4 KMNIST the statistics does not allow a clear analysis.

In Figure 2 we show the supremacy of the identified topological properties during the learning process for the FC4-KMNIST case.

| Architecture | Accuracy: $p_c$ | Accuracy: $\mu$ |
|---|---|---|
| FC4-MNIST | 0.00753(9) | 0.32(1) |
| FC4-KMNIST | 0.0075(1) | 0.29(2) |
| CNN5-MNIST | 0.00157(5) | 0.31(6) |
| CNN5-KMNIST | 0.00228(9) | 0.38(1) |
| | Pred. entropy: $p_c$ | Pred. entropy: $\theta$ |
| FC4-MNIST | 0.007187(8) | 0.15(2) |
| FC4-KMNIST | 0.0044(3) | 0.37(9) |
| CNN5-MNIST | 0.00079(4) | 0.12(8) |
| CNN5-KMNIST | 0.00152(4) | 0.18(2) |

TABLE I: Critical quantities for the various architectures, and physical quantities.
